# Supplementary material for: Iterative Augmentation of Visual Evidence for Weakly-Supervised Lesion Localization in Deep Interpretability Frameworks: Application to Color Fundus Images
Source: arXiv:1910.07373 ancillary file (2022-02-01)
Supplement: Supplementary file 1 [file Supplementary_materials.pdf]

# Supplementary Material

## Iterative augmentation of visual evidence for weakly-supervised lesion localization in deep interpretability frameworks

Cristina González-Gonzalo, Bart Liefers, Bram van Ginneken, Clara I. Sánchez

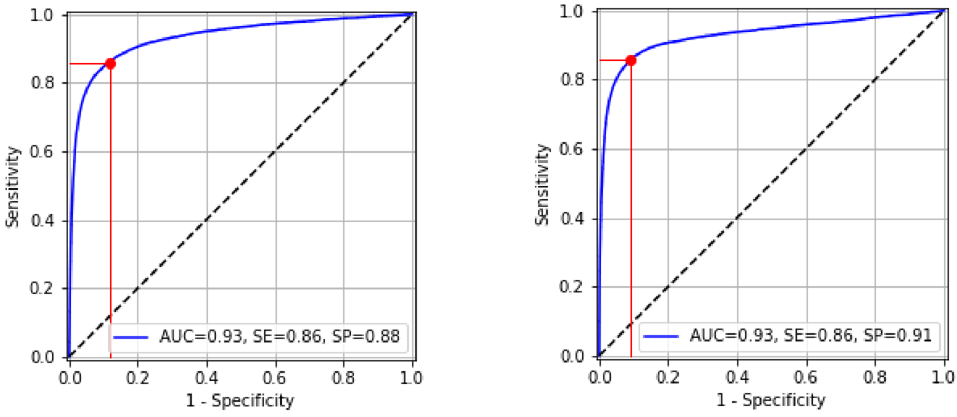


(a) (b)

Fig. S1. Receiver operating characteristic (ROC) curves for detection of referable diabetic retinopathy (DR) in the Kaggle test set (53,576 color fundus images) using the optimal DR classifier based on the VGG-16 architecture (a) and based on the Inception-v3 architecture (b). The red circles indicate the sensitivity (SE) and specificity (SP) of the classifiers at their optimal operating point, regarding the optimal threshold for referability obtained in the validation set. In (a), SE was 0.86, SP was 0.88, and the area under the ROC curve (AUC) was 0.93. In (b), SE was 0.86, SP was 0.91, and AUC was 0.93.

TABLE SI
OVERALL PERFORMANCE AND PERFORMANCE PER INDIVIDUAL MODEL IN THE AREDS DATASET

| Model | Test fold | | | | | | Evaluation metrics | | | |
|---|---|---|---|---|---|---|---|---|---|---|
| | Patients | Images | AMD stages (%) | | | | AUC | SE | SP | κ |
| | | | 0 | 1 | 2 | 3 | | | | |
| 1 | 922 | 27,027 | 8,231 (30.5) | 7,282 (26.9) | 7,883 (29.2) | 3,631 (13.4) | 0.97 | 0.90 | 0.92 | 0.86 |
| 2 | 923 | 27,108 | 8,795 (32.4) | 6,981 (25.8) | 8,142 (30.0) | 3,190 (11.8) | 0.97 | 0.89 | 0.93 | 0.86 |
| 3 | 923 | 26,665 | 8,060 (30.2) | 6,365 (23.9) | 8,365 (31.4) | 3,875 (14.5) | 0.97 | 0.92 | 0.90 | 0.88 |
| 4 | 923 | 26,836 | 8,177 (30.5) | 6,363 (23.7) | 8,754 (32.6) | 3,542 (13.2) | 0.97 | 0.90 | 0.92 | 0.86 |
| **5** | **922** | **26,184** | **8,146 (31.1)** | **6,001 (22.9)** | **8,351 (31.9)** | **3,686 (14.1)** | **0.97** | **0.92** | **0.93** | **0.88** |
| Global | 4,613 | 133,820 | 41,409 (30.9) | 32,992 (24.7) | 41,495 (31.0) | 17,924 (13.4) | 0.97 | 0.91 | 0.92 | 0.87 |

Five-fold cross-validation was used in the AREDS dataset (133,820 color fundus images from 4,613 patients) to obtain the optimal age-related macular degeneration (AMD) classifier. The number of patients was randomly divided in five groups and all the images of each patient were included in the corresponding fold. Each fold had an average number of 26,764 images, and AMD severity stages had a balanced distribution among folds. Four different evaluation metrics were computed to analyze the performance of each model in the corresponding test fold: area under the receiver operating characteristic curve (AUC), sensitivity (SE) and specificity (SP) at the optimal operating point regarding the optimal threshold for referability obtained in the corresponding validation fold, and quadratic Cohen's weighted kappa coefficient (κ). The last row includes the overall performance in the whole AREDS dataset. The model selected as optimal AMD classifier is indicated in bold.

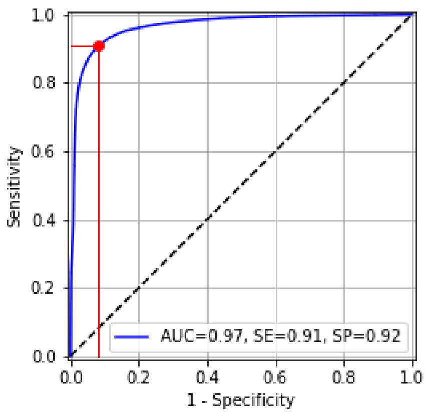


Fig. S2. Receiver operating characteristic (ROC) curve for detection of referable age-related macular degeneration (AMD) in the whole AREDS dataset (133,820 color fundus images), derived from the predictions made by the 5 models based on the VGG-16 architecture that were trained with 5-fold cross-validation (see Table S1). The red circle indicates the sensitivity (SE) and specificity (SP) at the optimal operating point. SE was 0.91, SP was 0.92, and the area under the ROC curve was 0.97.

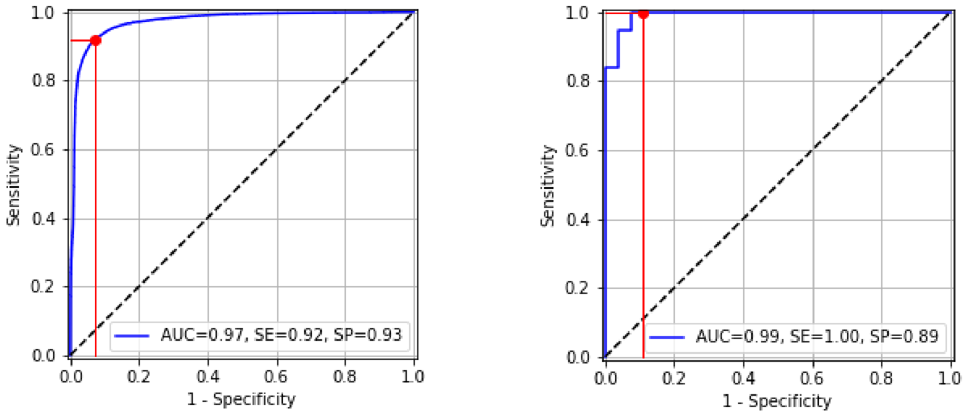


(a) (b)

Fig. S3. Receiver operating characteristic (ROC) curves for detection of referable age-related macular degeneration (AMD) using the optimal AMD classifier in the corresponding test fold (27,027 color fundus (CF) images) (a), and in the EUGENDA dataset (64 CF images) (b). The red circles indicate the sensitivity (SE) and specificity (SP) of the classifier at its optimal operating point in each dataset, regarding the optimal threshold for referability obtained in the validation set. In (a), SE was 0.92, SP was 0.93, and the area under the ROC curve (AUC) was 0.97. In (b), SE was 1.00, SP was 0.89, and AUC was 0.99.

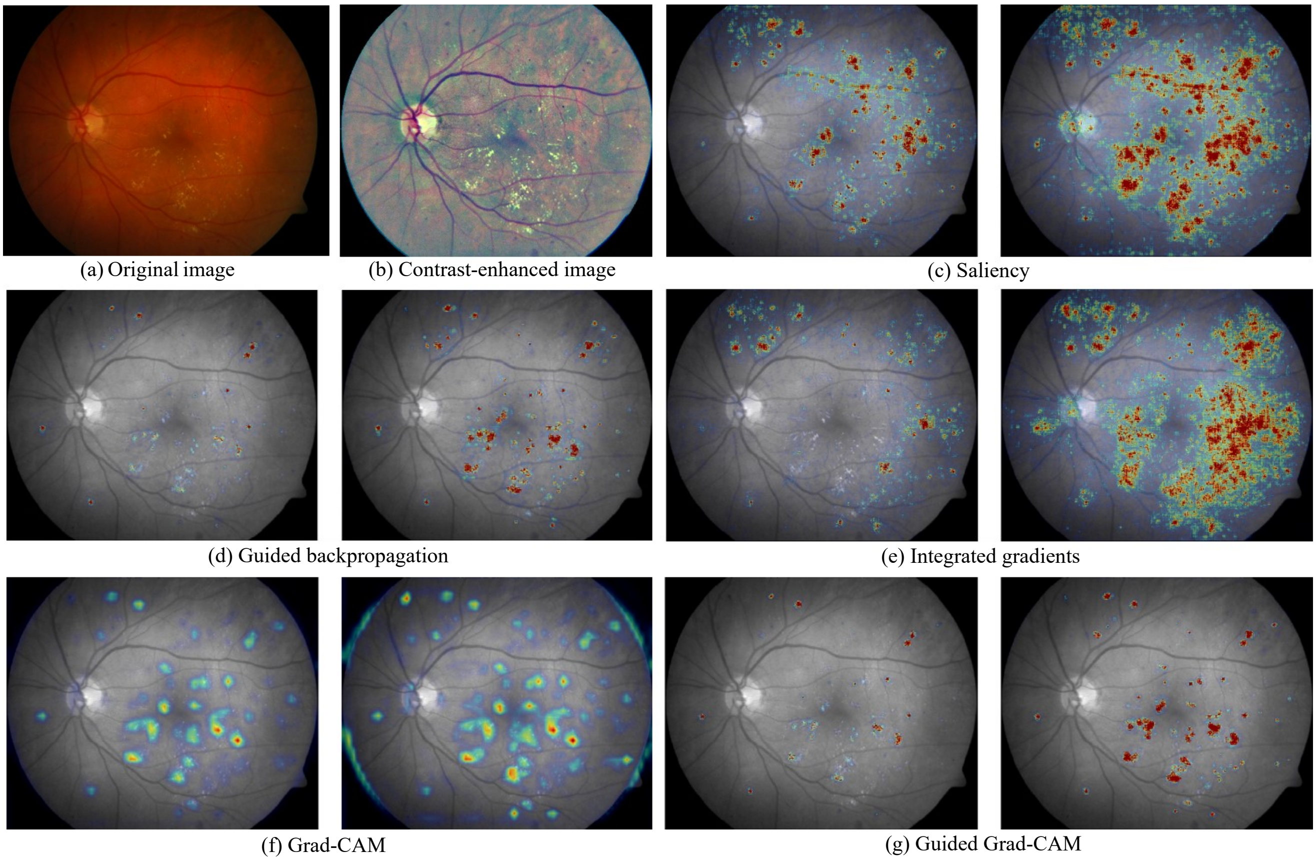


Fig. S4. Example of visual evidence generated with different methods for one image of DiaretDB1, predicted as DR stage 2 with the DR classifier based on VGG-16. For each method: initial visual evidence (left) and augmented visual evidence (right).

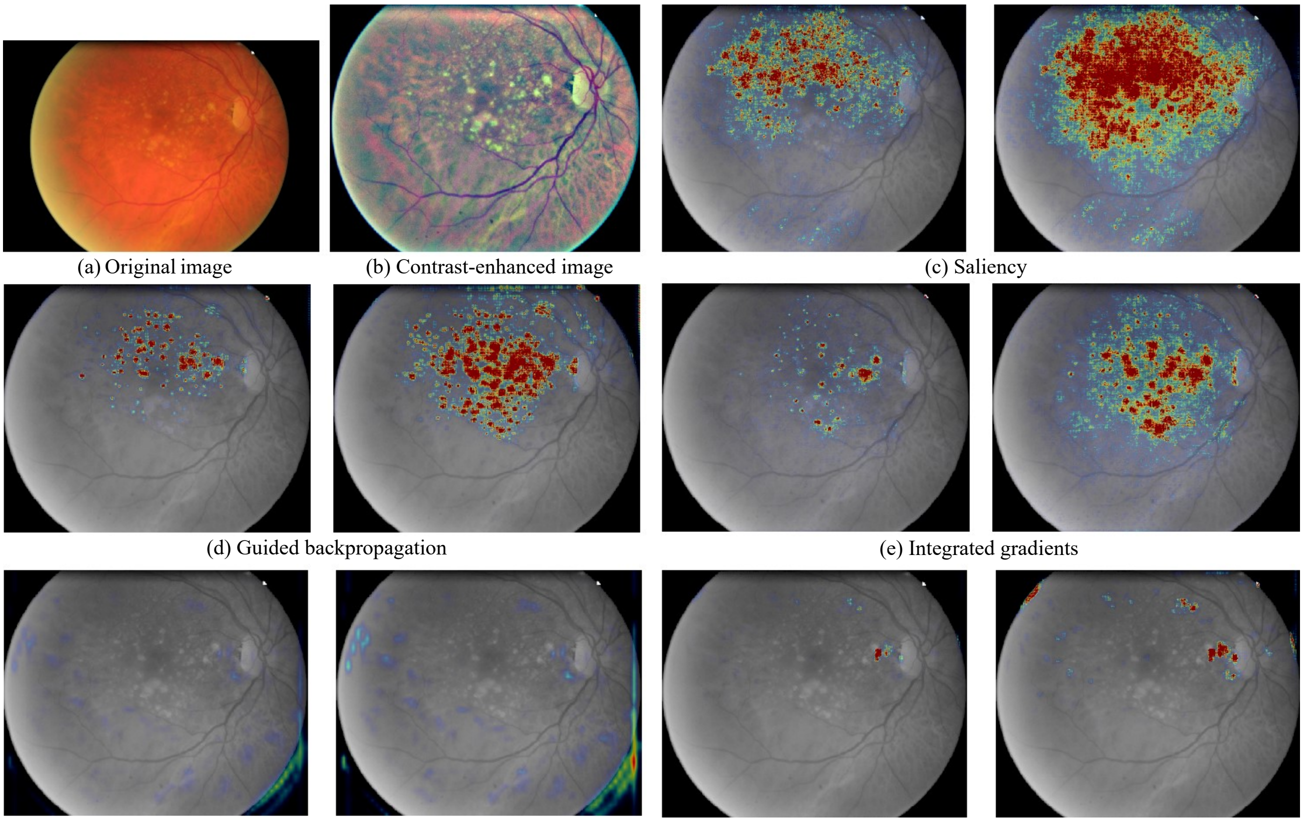

(a) Original image (b) Contrast-enhanced image (c) Saliency

(d) Guided backpropagation (e) Integrated gradients

(f) Grad-CAM (g) Guided Grad-CAM

Fig. S5. Example of visual evidence generated with different methods for one image of EUGENDA, predicted as AMD stage 2 (ground-truth label: AMD stage 2). For each method: initial visual evidence (left) and augmented visual evidence (right).
